# Supplementary material for: Hamiltonian cycles in Cayley graphs whose order has few prime factors
Source: arXiv:1009.5795 ancillary file (2011-04-04)
Supplement: Supplementary file 1 [file A5.pdf]

# CAYLEY GRAPHS ON $A_5$ ARE HAMILTONIAN

K. KUTNAR, D. MARUŠIČ, D. W. MORRIS, J. MORRIS, AND P. ŠPARL

This unpublished appendix to [28] provides a proof of Lemma 2.32 of that paper:

(2.32) **Lemma.** *Every connected Cayley graph on the alternating group $A_5$ has a hamiltonian cycle.*

Before the proof, we recall the following classical result:

(A1) **Theorem** (R. A. Rankin [29, Thm. 3.1(i)]). *If $\{a, b\}$ is a generating set of a finite group $G$, and $|ab| = 2$, then $\mathrm{Cay}\big(G; \{a, b\}\big)$ has a hamiltonian cycle.*

**Proof of Lemma 2.32.** Let $S$ be a minimal generating set of $G = A_5$.

**Case 1.** *Assume $\#S = 2$.* Write $S = \{a, b\}$.

**Subcase 1.1.** *Assume $|a| = 2$ and $|b| = 3$.* By applying an automorphism of $G$, we may assume $a = (1, 2)(3, 4)$ and $b = (2, 4, 5)$. A hamiltonian cycle is given by:

$$\big((a, b^{-2}, a, b^2)^2, (a, b^{-2})^3, (a, b^2)^3\big)^2.$$

**Subcase 1.2.** *Assume $|a| = 2$ and $|b| = 5$.* By applying an automorphism of $G$, we may assume $b = (1, 2, 3, 4, 5)$, and that $a$ is either $(1, 2)(3, 4)$, $(1, 3)(2, 4)$, or $(1, 4)(2, 3)$.

- If $a = (1, 2)(3, 4)$, then $|a| = 2$, $|b| = 5$, and $|ab| = 3$, so this is a $\langle 2, 5, 3\rangle$-presentation of $A_5 \cong \mathrm{PSL}_2(5)$, so [26] provides a hamiltonian cycle in $\mathrm{Cay}(G; S)$.
- If $a = (1, 3)(2, 4)$ then a hamiltonian cycle is given by:

$$\big((a, b^2)^2, a, b, a, b^{-2}, a, b, (a, b^{-1})^2, a, b^2, a, b^{-4}, a, b^{-2}, a, b,$$
$$a, b^{-1}, a, b^2, a, b^4, a, b^{-2}, (a, b)^2, a, b^{-1}, a, b^2, a, b^{-1}, (a, b^{-2})^2\big).$$

- If $a = (1, 4)(2, 3)$, then $a$ normalizes $b$, so $\langle a, b\rangle \neq G$, which contradicts the fact that $S$ is a generating set.

**Subcase 1.3.** *Assume $|a| = |b| = 3$.* By applying an automorphism of $G$, we may assume $a = (1, 2, 3)$ and $b = (3, 4, 5)$. A hamiltonian cycle is given by:

$$(a^{-2}, b, a, b^{-1}, a^{-2}, b^2, a^2, b, a, b^{-1}, a^2, b^{-1}, a^{-2}, b^2, a^{-2}, b^{-2}, a^{-2}, b^{-1}, a^2,$$
$$b^2, a^{-2}, b^{-2}, a^2, b, a^{-2}, b^2, a^2, b^{-2}, a^2, b^{-1}, a^{-2}, b^2, a^{-2}, b^{-2}, a^{-1}, b^{-1}).$$

**Subcase 1.4.** *Assume $|a| = 3$ and $|b| = 5$.* By applying an automorphism of $G$ (and perhaps replacing $a$ with its inverse), we may assume $b = (1, 2, 3, 4, 5)$, and that $a$ is either $(1, 2, 3)$ or $(1, 2, 4)$.

- If $a = (1, 2, 3)$, then a hamiltonian cycle is given by:

$$\big(b, a^{-1}, b, a^{-2}, b^{-2}, (a^2, b)^2, a^{-2}, b, a^{-2}, b^2, a^2, b^{-2}, (a^2, b^{-1})^2,$$
$$a^{-2}, b^{-1}, a^{-2}, b, a^{-1}, b, a^2, b^{-1}, a^2, b, a^{-2}, b^{-1}, a^{-1}, b^{-1}, (a^2, b^{-1})^2, a^{-2}, b^{-1}, a^{-2}\big).$$

- If $a = (1, 2, 4)$, then $a^{-1}b = (1, 5)(3, 4)$ has order 2, so Theorem A1 applies.

*Date*: March 2011.

**Subcase 1.5.** *Assume* $|a| = |b| = 5$. By applying an automorphism of $G$, we may assume $a = (1,2,3,4,5)$. We may assume $\{|ab|, |ab^{-1}|\} \subset \{3,5\}$, for otherwise Theorem A1 applies.

- If $|ab| = 3$, then, conjugating by a power of $a$, we may assume $ab$ is $(1,2,3)^{\pm 1}$ or $(1,2,4)^{\pm 1}$. Of the four resulting possibilities for $b = a^{-1}(ab)$, the only one with $|b| = 5$ and $|ab^{-1}| \neq 2$ is $b = (1,5,2,4,3)$. For these values of $a$ and $b$, a hamiltonian cycle is

$$\big(a^{-1}, b, a^4, b^{-1}, a^{-4}, b, a^4, b^{-2}, a^4, b^{-1}, a^{-1}, b^{-1},\\ a^3, b^{-1}, a^2, b, (a^4, b^{-1})^2, a^{-4}, b^{-1}, a^{-2}, b, (a^{-4}, b)^2\big).$$

- If $|ab^{-1}| = |ab| = 5$, then $b = (1,3,5,2,4)^{\pm 1} = a^{\pm 2}$. This contradicts the fact that $\langle a, b\rangle = A_5$.

**Case 2.** *Assume* $\#S \geq 3$. Since $S$ is minimal, it is easy to see that $\#S = 3$, so we may write $S = \{a, b, c\}$ with $|a| \leq |b| \leq |c|$.

**Subcase 2.1.** *Assume* $|c| = 5$. We may assume $a$ does not normalize $\langle c\rangle$. Then $\langle a, c\rangle = G$ (since every proper subgroup of $A_5$ whose order is divisible by 5 has order 5 or 10), which contradicts the minimality of $S$.

**Subcase 2.2.** *Assume* $|a| = |b| = |c| = 3$. Let $n = 5$. By applying an automorphism of $G$, and perhaps replacing some generators by their inverses, we may assume

$$S = \{(1,2,5), (1,3,5), (1,4,5)\} = \{\, (1,j,n) \mid 1 < j < n \,\}.$$

For this generating set (in any alternating group $A_n$), a hamiltonian cycle can be found in [27].

**Subcase 2.3.** *Assume* $|a| = 2$ *and* $|b| = |c| = 3$. Since $\langle b, c\rangle$ is a proper subgroup of $A_5$ that is generated by elements of order 3, it is conjugate to $A_4$. So we may assume $b = (1,2,3)$ and $c = (1,2,4)$. And then, since $S$ is minimal, we may assume $a = (1,2)(4,5)$ (perhaps after applying an automorphism of $G$ that interchanges $b$ and $c$). A hamiltonian cycle is given by

$$\Big((a, b, a, b^{-1}, a, c)^3, (a, b, a, b^{-1}, a, c^{-1})^3\#, c, a, c^{-1}, a, b^{-1},\\ a, b, a, c^{-1}, (a, b, a, b^{-1}, a, c^{-1})^2\#, c, a, b^{-1}, a, c^{-1}\Big)$$

**Subcase 2.4.** *Assume* $|a| = |b| = 2$ *and* $|c| = 3$. We may assume $c = (1,2,3)$.

- If $a$ interchanges 4 and 5, then we may assume $a = (1,2)(4,5)$. And then we may assume $b$ is either $(1,2)(3,4)$ or $(1,3)(2,4)$.
  - If $b = (1,2)(3,4)$, a hamiltonian cycle is given by:

$$\Big(a, c, a, b, c^{-1}, a, c^{-2}, (a, b)^2, c, a, c^2, a, b, c^2, b, c, a, c, b, a, c^{-1}, a, c, a,\\ b, c^{-1}, a, c^{-2}, a, b, c^2, b, a, c^{-1}, a, c, a, b, c^{-1}, a, c^{-2}, a, b, a, c^2, a, c, b, a, c^{-1}\Big)$$

  - If $b = (1,3)(2,4)$, a hamiltonian cycle is given by:

$$\Big(\big((a, b)^4, c, b\big)^2\#, c, (a, b)^4, a, c^{-2}, b, (a, b)^4, c^{-1}, (b, a)^4, c, (a, b)^4, a, c^{-1}\Big)$$

- If neither $a$ nor $b$ interchanges 4 and 5, then one of them must fix 4, and the other must fix 5. We may assume $a = (1,2)(3,4)$. And then we may assume $b$ is either $(1,2)(3,5)$ or $(1,3)(2,5)$.
  - If $b = (1,2)(3,5)$, a hamiltonian cycle is given by:

$$\Big(\big((a,b)^2, a, c\big)^2\#, c^{-1}, (a,b)^2, a, c^2, b, (a,b)^2, c^{-2}, b, (a,b)^2,$$
$$c^2, b, (a,b)^2, c^{-1}, \big((b,a)^2, c\big)^2\#, b, c^{-1}, a, b, (a,b,a,c)^2\#, c^{-1}\Big)$$

  - If $b = (1,3)(2,5)$, a hamiltonian cycle is given by:

$$\big(a, c^{-1}, (a,b)^2, c, b, (a,b)^4, c^{-1}, (b,a)^2, c, (a,b)^4\big)^2$$

**Subcase 2.5.** *Assume* $|a| = |b| = |c| = 2$. In this case, since $S$ generates $A_5$, it is not difficult to see that some pair of elements of $S$ generates a transitive subgroup. So we may assume $\langle a, b\rangle$ is transitive, which means that, up to isomorphism, we have $a = (1,2)(3,4)(5)$ and $b = (1,5)(2,3)(4)$.

Conjugation by the permutation $\sigma = (1,3)(4,5)$ interchanges $a$ and $b$, so we may assume the fixed point of $c$ is either 1, 2, or 4 (after conjugating by $\sigma$ if necessary). We now provide a hamiltonian cycle for each possible choice of $c$:

- $c = (2,3)(4,5)(1)$: $\big((a,b)^4, c, (a,b)^2, c, (a,b)^4, a, c, (b,a)^2, c, b\big)^2$
- $c = (2,4)(3,5)(1)$: $\{a,b,c\} \subset N_G\big(\langle(1,2,3,5,4)\rangle\big)$ does not generate $A_5$.
- $c = (2,5)(3,4)(1)$: $\big((b,a)^3, b, c, (b,a)^4, (b,c)^2\big)^3$
- $c = (1,3)(4,5)(2)$: $\{a,b,c\} \subset N_G\big(\langle(1,2,3,5,4)\rangle\big)$ does not generate $A_5$.
- $c = (1,4)(3,5)(2)$:

$$\Big(\big((a,b)^4, c, b\big)^2, a, (b,c)^2, (b,a)^2, c, b, a, b, c, (a,b)^4, a, c, b, a, b, c, (a,b)^2, (c,b)^2, a, b, c, b\Big)$$

- $c = (1,5)(3,4)(2)$: $\big((a,b)^3, (c,b)^2, (a,b)^4, c, b\big)^3$
- $c = (1,2)(3,5)(4)$:

$$\Big(\big((a,b)^4, c, b\big)^2, (a,b)^2, c, b, (a,b)^4, c, (b,a)^2, c, (a,b)^4, a, c, (a,b)^2, c, b, a, b, c, b\Big)$$

- $c = (1,3)(2,5)(4)$:

$$\big((a,b)^3, a, c, (a,b)^2, a, c, (a,b)^4, a, c, a, b, (a,c)^2,$$
$$(a,b)^2, a, c, (a,b)^3, a, c, (a,b)^4, (a,c)^2, a, b, a, c\big) \qquad \square$$

## Additional references


[26] H. H. Glover and T. Y. Yang: A Hamilton cycle in the Cayley graph of the $\langle 2, p, 3\rangle$ presentation of $\mathrm{PSL}_2(p)$, *Discrete Math.* 160 (1996), no. 1–3, 149–163.

[27] R. J. Gould and R. L. Roth: A recursive algorithm for Hamiltonian cycles in the $(1, j, n)$-Cayley graph of the alternating group, in Y. Alavi et al., eds.: *Graph Theory with Applications to Algorithms and Computer Science (Kalamazoo, Mich., 1984)*. Wiley, New York, 1985, pp. 351–369.

[28] K. Kutnar, D. Marušič, J. Morris, D. W. Morris, and P. Šparl: Hamiltonian cycles in Cayley graphs whose order has few prime factors, *Ars Mathematica Contemporanea* (to appear). http://arxiv.org/abs/1009.5795

[29] R. A. Rankin: A campanological problem in group theory II, *Proc. Cambridge Philos. Soc.* 62 (1966) 11–18.
